# Supplementary material for: Blind Identification of Fully Observed Linear Time-Varying Systems via Sparse Recovery
Source: arXiv:1712.10095 source file (2018-05-21)
Supplement: Supplementary file 1 [file appendices.tex]

\section{Sparse Recovery Theory}
\label{sec:AppendixSRT}
(NB: This Appendix is added to support the reviewer by providing theory with symbols similar as in the main manuscript. It can be omitted in the event of publication)
\subsection{Theory for Fully Sparse Support}
\label{sec:AppendixSRTa}
In the last decade, a rich body of new literature has formed to address the equivalence and exact recovery of compressed sensing problems, i.e. determining under what conditions the solution to \eqref{eq:CSP1} is equivalent and exactly recovers the solution to the NP-hard problem \eqref{eq:CSP0}. Here, we first address the results for noiseless case.
Exact recovery is generally assessed through inspection of the \emph{spark} property or, more practically, through the \emph{Mutual Coherence Condition} (MCC) of the sensing matrix $\Psi$.
The review paper \cite{bruckstein_sparse_2009} provides a solid overview of the theoretical principles developed for the canonical problem, in which the support of the solution vector is fully sparse. 
The following lemma enables the equivalence of solution between the non-convex compressed sensing problem and its convex relaxation.
Consider problem $P_1$ as introduced in \eqref{eq:CSP1}, with sensing matrix $\Psi \in \R^{m \times D}$.
\begin{definition}
The spark of a matrix $\Psi$ is the smallest number of columns of $\Psi$ that are linearly dependent.
\end{definition}
\begin{definition}
The mutual coherence of a matrix $\Psi$ is the largest absolute normalized inner product between different columns from $\Psi$. Denoting the $k$-th column in $\Psi$ by $p_k$, the mutual coherence is given by
\begin{equation}
\mu(\Psi) = \displaystyle \max_{1 \le k,j \le N , k \ne j} \dfrac{\left| p_k^{\top} p_j \right| }{\| p_k \|_2 \cdot \| p_j \|_2} 
\end{equation}
\end{definition}
Given these definitions, the following lemma adopted from \cite{bruckstein_sparse_2009} provides sufficient conditions for equivalence between the compressed sensing problem $P_0$ \eqref{eq:CSP0} and its convex relaxation $P_1$ \eqref{eq:CSP1}.
\begin{lemma} 
\label{lm:MCC}
(Equivalence - Spark and Mutual Coherence Condition)
For the system of linear equations $\Psi x = b$ ($\Psi \in \R^{D \times N}$ full-rank with $D < N$), if a solution $x$ exists obeying
\begin{equation}
\| x  \|_0 < \frac{1}{2}\left( 1 + \frac{1}{\mu(\Psi)}  \right) \le \frac{1}{2} \text{spark} (\Psi),
\end{equation}  
that solution is both the unique solution to the convex relaxation \eqref{eq:CSP1}, and the unique solution to the original NP-hard compressed sensing problem \eqref{eq:CSP0}.
\end{lemma}
The original proof was derived for the spark condition. The mutual coherence condition (MCC) provides a lower bound on the spark condition, for which a lemma is provided in \cite{bruckstein_sparse_2009}. The MCC is typically used as spark is expensive to compute. 
Notice that this result does not guarantee existence, but only provides the equivalence between solutions for the original problem \eqref{eq:CSP0} and its convex relaxation \eqref{eq:CSP1}.

Existence and uniqueness of the convex relaxation problem (our target problem) can be assessed through two different properties - the \emph{Null Space Property} (NSP), and the \emph{Restricted Isometry Property} (RIP) of the sensing matrix $\Psi$.
This theory was originally developed in \cite{donoho_optimally_2003} (NSP) and \cite{candes_restricted_2008} (RIP) for problems that have a solution with a fully sparse support. Here, we briefly state available theory that provides guarantees for extending these notions to scenarios with partial sparse support, which is critical to our problem formulation \eqref{eq:noiselessCS}. As assumed before, here we again need $\Psi_a$ to be full column rank.

Some notation: For sake of brevity, let $N = n k_f q + n^2 k_f$ be the dimension of our solution vector $[\pmb{u}^{\top} \ \pmb{a}^{\top} ]^{\top}$, and let $s$ denote its number of nonzero entries. Let $[N]$ represent the set of integers $\{ 1, 2, \hdots, N \}$, and $[N]^{(s)}$ the set of all subsets of $[N]$ of cardinality $s \le N$. Given $ \pmb{x} =  \in \R^N$ and $S \in [N]$, $x_S \in \R^N$ denotes a vector defined by $(\pmb{x}_S)_i = \pmb{x}_i , i \in S$ and $(\pmb{x}_S)_ i = 0 , i \notin S$. 
\begin{definition} (Null Space Property)
A matrix $\Psi \in \R^{D \times N}$ satisfies the Null Space Property (NSP) of order $s$ for  sparse recovery of size $N$ if, for every $\pmb{x} \in \R^{N}_{\backslash \{0\}}$ and every $S \in [N]^{(s)}$, we have
\begin{equation}
\| \pmb{x}_S \|_1 < \frac{1}{2} \| \pmb{x} \|_1
\end{equation}
\end{definition}
 
\begin{lemma} (NSP $\iff$ unique sparse recovery) The matrix $\Psi$ satisfies the Null Space Property of order $s$ if and only if, for every true $s$-sparse vector $\bar{\pmb{x}} = [\bar{\pmb{u}}^{\top} \ \bar{\pmb{a}}^{\top} ]^{\top} $, \eqref{eq:CSP1} with $\pmb{z} = \Psi \bar{\pmb{x}}$ has a unique solution given by $\pmb{x} = \bar{\pmb{x}}$. 
\label{thm:NSPunique}
\end{lemma}
 
\begin{definition} (Restricted Isometry Property)
A scalar $\delta_s > 0$ is the Restricted Isometry Property (RIP) constant of order $s$ of the matrix $\Psi \in \R^{D \times N}$ if it is the smallest positive real number such that
\begin{equation}
(1 - \delta_s) \| \pmb{x} \|_2^2 \le \| \Psi \pmb{x} \|_2^2 \le (1 + \delta_s) \| \pmb{x} \|_2^2
\end{equation}
for every $s$-sparse vector $\pmb{x}$.
\label{def:RIP}
\end{definition}

\begin{lemma} (RIP $\iff$ unique sparse recovery)
Let $\Psi \in \R^{D \times N}$ and $2s < D$. If $\delta_{2s} < \sqrt{2} - 1$, where $\delta_{2s}$ is the RIP constant of $\Psi$ of order $2s$, then the convex relaxation \eqref{eq:CSP1} with $\pmb{z} = \Psi \bar{\pmb{x}}$ has a unique solution given by $\pmb{x} = \bar{\pmb{x}}$, for every $s$-sparse vector $\bar{\pmb{x}}$.
\label{thm:RIPunique}
\end{lemma} 

In many realistic contexts, the measurement vector $y$ (as in \eqref{eq:CSP1}) contains noise and the signal $s$ is not sparse but \emph{compressible}. This means that many components are very small but not necessarily zero. Theoretical advances have generalized the Compressive Sensing framework to be robust to noise and recover compressible signals \cite{candes_restricted_2008}. 

\begin{lemma} 
\label{thm:compressible}
(Recovery of Compressible Signals) Assume that the matrix $\Psi \in \R^{m \times D}$ satisfies the RIP condition in Lemma \ref{thm:RIPunique} with RIP constant $\delta_{2s} < \sqrt{2} - 1$. For any true signal $\bar{x} \in \R^D$, let the noisy measurement be $y = \Psi \bar{x} + w$, with $\| w \|_2 \le \eta$. Let $x^*$ be a solution of 
\begin{equation}
P_2 \ : \ \displaystyle \min_{x \in \R^D} \| x \|_1 \quad \text{subject to} \quad \| \Psi x - y \|_2 \le \eta.
\end{equation}
Then it follows that the solution is close to the true signal as given by
\begin{equation}
\| x^* - \bar{x} \|_2 \le \alpha_1 \eta + \alpha_2 \dfrac{\sigma_s (\bar{x})_1}{\sqrt{s}},
\label{eq:stability1}
\end{equation}
with constants $\alpha_1,\alpha_2$ depending on RIP constant $\delta_{2s}$, and $\sigma_s (\bar{x})_1 = \min_{x : \| x \|_0 \le s} \| x - \bar{x} \|_1$.
\end{lemma}
The proof for this lemma can be found in \cite[Theorem 5.1]{bandeira_partial_2013}.

%%%%%%%%%%%%%%%%%%%%%%%%%%%%%%%%%%%%%%%%%%%%%%%%%%%%%%%%%%%%%%%%%%%%%%%%%%%%%%%%%%%%%%%%%%%%%%%%%%%%%%%%%%%%%%%%%%%%

\subsection{Extension to Partially Sparse Support}
\label{sec:AppendixSRTb}
Several independent works have addressed the generalization to solutions for which part of the support of the solution $x$ is known \cite{bandeira_partial_2013,friedlander_recovering_2012,jacques_short_2010,vaswani_modified-cs:_2010}. The authors in \cite{bandeira_partial_2013} have focused their theory on the case where an a priori known part of the support of the solution is known to be dense, which relates to our problem formulation \eqref{eq:noiselessCS}, for which $\pmb{a}$ is generally a dense vector. 
We adopt two lemmas that outline these properties for partially sparse compressed sensing problems.

Let $r$ denote the number of entries in the dense part of our solution vector, i.e. $r = \text{dim}(\pmb{a}) = n^2 k_f$ (or $n^2$ in the LTI case).
\begin{definition} (Partial Null Space Property)
Our sensing matrix $\Psi = [\Psi_u \ | \ \Psi_a] \in \R^{D \times N}$ satisfies the Null Space Property (NSP) of order $s - r$ for partially sparse recovery of size $N - r$ with $r \le s$ if $\Psi_a$ is full column rank and for every $\pmb{u} \in \R^{N-r}_{\backslash \{0\}}$ such that $\Psi_u \pmb{u} \in \CMcal R (\Psi_a)$ and every $S \in [N - r]^{(s-r)}$, we have
\begin{equation}
\| (\pmb{u})_S \|_1 < \frac{1}{2} \| \pmb{u} \|_1
\end{equation}
\end{definition}
\begin{lemma} (Partial NSP $\iff$ uniqueness - adopted from \cite{bandeira_partial_2013})
The matrix $\Psi = [\Psi_u \ | \ \Psi_a] \in \R^{D \times N}$ satisfies the Null Space Property (NSP) of order $s - r$ for partial sparse recovery of size $N - r$ if and only if for every $\bar{\pmb{x}} = ( \bar{\pmb{x}}_1 , \bar{\pmb{x}}_2)$ such that $\bar{\pmb{x}}_1 \in \R^{N-r}$ is an $s-r$ sparse vector and $\bar{\pmb{x}}_2 \in \R^{r}$, problem \eqref{eq:noiselessCS} with $\pmb{z} = \Psi_u \pmb{u} +  \Psi_a \pmb{a}$ has a unique solution given by $(\pmb{u} , \pmb{a}) = (\bar{\pmb{x}}_1 ,\bar{\pmb{x}}_2)$.
\end{lemma} 
\begin{definition} (Partial RIP - adopted from \cite{bandeira_partial_2013})
$\delta_{s-r}^r > 0$ is the Partial Restricted Isometry Property Constant of order $s - r$ of the matrix $\Psi = [\Psi_u \ | \ \Psi_a] \in \R^{D \times N}$, for recovery of size $N - r$ with $r \le s$, if $\Psi_a$ is full column rank and $\delta_{s-r}^r$ is the RIP constant of order $s - r$ (see Definition \ref{def:RIP}) of the matrix $\CMcal P \Psi_u$, where $\CMcal P$ is given by \eqref{eq:proj}.
\end{definition}  

Notice that with $r = 0$ the Partial RIP reduces to the RIP of Definition \ref{def:RIP}. 
Combining Theorems \ref{thm:NSPunique} and \ref{thm:RIPunique}, one can show that, given a matrix $\Psi = [\Psi_u \ | \ \Psi_a] \in \R^{D \times N}$ with Partial RIP constant $\delta_{2(s-r)}^r$ of order $2(s-r)$ for recovery of size $N - r$, satisfying $\delta_{2(s-r)}^r < \sqrt{2} - 1$, $\CMcal P \Psi_u$ satisfies the NSP property of order $s - r$. 
Hence, given a true signal $\bar{\pmb{x}} = (\bar{\pmb{x}}_1,\bar{\pmb{x}}_2)$ such that $\bar{\pmb{x}}_1$ is $(s-r)$-sparse and $\bar{\pmb{x}}_2 \in \R^{r}$, $\bar{\pmb{x}}_1$ can be recovered by minimization of the $\ell_1$-norm of $\pmb{u}$ subject to $(\CMcal P \Psi_u)\pmb{u} = \CMcal P \Psi [\pmb{u}^{\top} \ \pmb{a}^{\top} ]^{\top}$ and, since $\Psi_a$ is assumed to be full column rank, $\pmb{a} = \bar{\pmb{x}}_2$ is uniquely determined by $\Psi_a \pmb{a} = \pmb{z} - \Psi_u \pmb{u} = \pmb{z} - \Psi_u \bar{\pmb{x}}_1$ \cite{bandeira_partial_2013}. In other words, this implies that $\Psi$ satisfies the NSP of order $s - r$ for partially sparse recovery of size $N - r$.

In short, we see that if we assume that $\Psi_a$ is full column rank and the sensing matrix $\Psi$ satisfies the NSP (Lemma \ref{thm:NSPunique}) or RIP (Lemma \ref{thm:RIPunique}) property, our problem \eqref{eq:noiselessCS} with partial sparse support will have a unique solution for any true signal $\bar{\pmb{x}}$.

Lastly, consider the result for retrieving a compressible signal in \eqref{thm:compressible}.
In our scenario the support of the true signal $\bar{x} = [\bar{x}_1^{\top} \ \bar{x}_2^{\top}]^{\top} $ is only partially sparse, i.e. $\bar{x}_2 \in \R^r$ is a dense vector. The following lemma extends Lemma \ref{thm:compressible} to this scenario.
\begin{lemma} (Recovery of Compressible Signals with Partially Sparse Support)
\label{thm:partialsparse_stability}
Since $\CMcal P$, as in \eqref{eq:proj}, is a projection matrix, we have that $\| \CMcal P \Psi_1 \bar{x}_1 - \CMcal P y \|_2 = \| \CMcal P \Psi \bar{x} - \CMcal P y \|_2 \le \| \Psi \bar{x} - y \|_2 \le \eta$, and the solution $x^*$ of 
\begin{equation}
P_3 \ : \ \displaystyle \min_{x_1 \in \R^{D-r}} \| x_1 \|_1 \quad \text{subject to} \quad \| \CMcal P \Psi_1 x_1 - \CMcal P y \|_2 \le \eta
\end{equation}
satisfies
\begin{equation}
\| x_1^* - \bar{x}_1 \|_2 \le \beta_1 \eta + \beta_2 \dfrac{\sigma_{s-r} (\bar{x}_1)_1}{\sqrt{s-r}},
\label{eq:stability2}
\end{equation}
where $\beta_1,\beta_2$ now depend on the RIP constant. $x^*_2$ is determined by $\Psi_2 x^*_2 = y - \Psi_1 x^*_1$, and obeys:
\begin{equation}
\| x_2^* - \bar{x}_2 \|_2 \le C_2 \left( 2 \eta + C_1 \left( \beta_1 \eta + \beta_2 \dfrac{\sigma_{s-r} (\bar{x}_1)_1}{\sqrt{s-r}} \right) \right),
\label{eq:stability_a}
\end{equation}
where $C_1 = \| \Psi_1 \|_2$ and $C_2 = \| \Psi^{\dagger}_2 \|_2$, with $\Psi^{\dagger}_2 = (\Psi^{\top}_2 \Psi_2)^{-1}\Psi^{\top}_2$.
\end{lemma}
The proof for this lemma can be found in \cite[Theorem 5.2]{bandeira_partial_2013}.
